# Supplementary material for: LTLf Adaptive Synthesis for Multi-Tier Goals in Nondeterministic Domains
Source: arXiv:2504.20983 source file (2025-04-29)
Supplement: Supplementary file 1 [file supplementary.tex]

\newpage
% \phantom{bla}
% \newpage

\section{Supplementary Material (Paper \#38)~\label{sec:supplementary}}

% cosa facciamo di preciso in questa sezione?
% what do we in do in this section?
In this section, we present the proof of Theorem~\ref{thm:multi-tier-correct}, i.e., correctness of Algorithm~\ref{alg:super-mega-iper-ultra-multi-tier}, thus
% cosa comporta precisamente questo risultato?
% what does this imply?
proving: \begin{enumerate}
    \item The strategy returned by Algorithm~\ref{alg:super-mega-iper-ultra-multi-tier} always satisfies Definition~\ref{def:best-effort-plan}, hence being an adaptive strategy;
    \item A solution strategy to adaptive synthesis for \LTLf multi-tier goals (Definition~\ref{def:best-effort-plan}) always exists (Theorem~\ref{thm:existence}).
\end{enumerate}

% quale è di preciso il primo passo che dobbiamo fare?
% what is the first step that we must take?
First, we review some results from the body of the paper and fix the notation. 
% quale è di preciso il primo risultato che rivediamo?
% what is the first result we review?
We recall: \begin{itemize}
    \item From Section~\ref{sec:preliminaries}: we can equivalently define agent strategies as $\sigma: (2^\F)^+ \rightarrow \act$ or $\sigma': (\react)^* \rightarrow \act$ in the planning domains we consider;
    \item From Section~\ref{sec:games}: game strategies $\kappa: Q \rightarrow \act$ induce agent strategies of the form $\sigma': (\react)^* \rightarrow \act$ (see Definition~\ref{dfn:induced-strategy}). 
\end{itemize}

% che cosa possiamo concludere di preciso da questi due risultati?
% what can we deduce by these two results?
Having in mind these two results, we will sometimes blur the technical distinction between strategies \mbox{$\sigma: (2^\F)^+ \rightarrow \act$} and \mbox{$\sigma': (\react)^* \rightarrow \act$} and \mbox{$\kappa: Q \rightarrow \act$} to simplify the notation.

% quale è il secondo risultato che richiamiamo dal corpo del paper?
% what is the second result that we recall from the body of the paper?
We now review some results about the notion of product of transition systems of a domain $\P_+$ and of the \DFA $\A_{\varphi}$ of an \LTLf objective $\varphi$ given in Definition~\ref{def:product-2}, here denoted {$\T = \textsc{Product}(\P_+, \A_{\varphi})$}.

Let $\tau = s_0(a_1, r_1, s_1) \cdots (a_n, r_n, s_n)$ be a legal trace of $\P$. 
% quale è di preciso il risultato che abbiamo per T e tau?
Running $\tau|_{\act \times \react}$ on $\T$ leads to state $t(\tau) = (s_n, \varrho(\iota, s_0 s_1 \cdots s_n))$, i.e.,
% quale è di preciso l'informazione contenuta nello stato
a pair consisting of the state $s_n$ reached in the domain
and the state $\varrho(\iota, s_0 s_1 \cdots s_n))$ reached in $\A_\varphi$ by reading the entire sequence of states $s_0 s_1 \cdots s_n$. As a result, legal histories $\tau$ correspond to paths of $\T$ not leading to any error state.
% per la direzione inversa cosa possiamo dire di preciso?
An analogous result holds in the converse direction, i.e., paths of $\T$ not leading to any error state corresponds to legal traces of $\P$. 
% e invece cosa possiamo dire di preciso riguardo alle traccie non legali?
% what about non-legal traces?
If $\tau$ is instead a non-legal trace, running $\tau|_{(\act \times \react)}$ in $\T$ will reach either $(\agerr, q)$ or $(\enverr, q)$, depending on which player violated its respective precondition. 
% e infine cosa possiamo dire di preciso riguardo l'altra direzione?
Similarly, paths of $\T$ leading to some error state correspond to non-legal traces of $\P$.

% quale è di preciso il prossimo passo?
We prove Theorem~\ref{thm:multi-tier-correct} by concatenating several intermediate results, which we discuss below. We first review the following result from~\cite{DPZ23Ecai}:

\begin{lemma}~\label{lem:games-to-histories}\cite{DPZ23}
    Let $\P$ be a domain and $\varphi$ an \LTLf objective. Denote with $t$ states of the transition system $\T$ computed in Step~3 of Algorithm~\ref{alg:single-goal-be}. 
    Let $(\w, \kappa)$ (resp. $(\c, \nu)$) be the winning region and uniform winning game strategy (resp. cooperative region and uniform positional cooperative strategy) computed in Line~9 (resp. Step~10) of Algorithm~\ref{alg:single-goal-be}. The following hold: \begin{enumerate}
        \item For every $h \in \H_\P$: \\ \centerline{if $\val{\varphi|\P}(h) = \win$, then $t(h) \in \w$}
        \item For every $h \in \H_\P$: \\ \centerline{if $\val{\varphi|\P}(h) = \pend$: then $t(h) \in \c \setminus \w$}
        \item For every $h \in \H_{\P}(\kappa)$: \\ \centerline{if $t(h) \in \w$, then $\val{\varphi|\P}(\kappa, h) = \win$}
        \item For every $h \in \H_{\P}(\nu)$: \\ \centerline{if $t(h) \in \c \setminus \w$, then $\val{\varphi|\P}(\nu, h) = \pend$}
    \end{enumerate}
\end{lemma}

\subsection{Proof of Theorem~\ref{thm:win-pend-strategy}}

As an intermediate step towards proving Theorem~\ref{thm:multi-tier-correct}, we prove Theorem~\ref{thm:win-pend-strategy}, which establishes the correctness of Algorithm~\ref{alg:strong-weak-plan} and is reported below for convenience. 

\setcounter{theorem}{+2}
\begin{theorem}~\label{thm:win-pend-strategy}
    Let $\P$ be a domain, $\varphi_1$ and $\varphi_2$ two \LTLf objectives such that $\L_{\P}(\varphi_{1}) \supseteq \L_{\P}(\varphi_{2})$, and $\sigma$ the strategy returned by Algorithm~\ref{alg:strong-weak-plan}. For every $h \in \H_{\P}(\sigma)$, if $\val{\langle \varphi_1,\varphi_2 \rangle|\P}(h) = \langle \win, \pend \rangle$, either: \begin{enumerate}[noitemsep,topsep=0pt,parsep=0pt,partopsep=0pt]
        \item 
        $\val{\langle \varphi_1, \varphi_2 \rangle|\P}(\sigma, h) = \langle \win, \pend \rangle$; or
        % \item 
        % $\val{\varphi_1|\P}(\sigma, h) = \win$.
        \item 
        If no agent strategy $\eta$ exists s.t. $\val{\langle \varphi_1, \varphi_2 \rangle|\P}(\eta, h) = \langle \win, \pend \rangle$, then $\val{\varphi_1|\P}(\sigma, h) = \win$.
    \end{enumerate}
\end{theorem}

To prove Theorem~\ref{thm:win-pend-strategy} we use the following: 

\begin{lemma}~\label{lem:strong-weak-plans}
    Let $\P$ be a domain and $\varphi$ an \LTLf objective. Let $\w_1$ and $\c_2$ be the regions computed in Lines 3-4 of Algorithm~\ref{alg:strong-weak-plan} and $\w_2 = \textsc{SolveAdv}(\T_2, Adv_2)$. Denote with $(t_1, t_2)$ states in the transition system $\T$ computed in Line~5 of Algorithm~\ref{alg:strong-weak-plan}.
    Let $(\wc, \sigma)$ be the region and strategy returned in Line 10 of Algorithm~\ref{alg:strong-weak-plan}.
     %, and let $(\wc, \sigma)$ be the returned region and the strategy. 
    The following hold: \begin{enumerate}
        \item For every $h \in \H_\P$: \\ \centerline{if $\val{(\varphi_1, \varphi_2)|\P}(h) = \langle \win, \pend \rangle$} \\ \centerline{then $(t_1(h), t_2(h)) \in \w_1 \times (\c_2 \setminus \w_2)$}
        \item For every history $h \in \H_{\P}(\sigma)$: \\ \centerline{if $(t_1(h), t_2(h)) \in \wc \cap (\w_1 \times (\c_2 \setminus \w_2))$} \\ \centerline{then $\val{(\varphi_1, \varphi_2)|\P}(\sigma, h) = \langle \win, \pend \rangle$}
        \item For every $h \in \H_\P$: \\ \centerline{if $(t_1(h), t_2(h)) \in (\w_1 \times (\c_2 \setminus \w_2)) \setminus \wc$} \\ \centerline{then: \textbf{(A)} $\neg \exists \eta$ such that: $\val{(\varphi_1,\varphi_2)|\P}(\eta, h) = \langle \win, \pend \rangle$}  \\\centerline{and \textbf{(B)} $\val{\varphi_1|\P}(\sigma, h) = \win$}
    \end{enumerate}
\end{lemma}

\begin{proof}[Proof of Lemma~\ref{lem:strong-weak-plans}]

We prove Item 1. Recall that $\val{(\varphi_1, \varphi_2)|\P}(h) = \langle \win, \pend \rangle$ is an abbreviation for $\val{\varphi_1|\P}(h) = \win$ and $\val{\varphi_2|\P}(h) = \pend$. By Items~1 and~2 in Lemma~\ref{lem:games-to-histories}, we have that $t_1(h) \in \w_1$ and $t_2(h) \in \c_2 \setminus \w_2$. Being $\T$ obtained by product, we have that $(t_1(h), t_2(h)) \in \w_1 \times (\c_2 \setminus \w_2)$.

We prove Item 2. First, we prove the following: \begin{itemize}
    \item[$(\dagger)$] for every $h \in \H_{\P}(\sigma)$: if $(t_1(h), t_2(h)) \in \wc$, then $\val{(\varphi_1, \varphi_2)|\P}(\sigma, h) \in \{\langle \win, \win \rangle, \langle \win, \pend \rangle\}$.
\end{itemize} 

We prove the claim by induction on stages of the fixpoint computation for $\wc$. For the base step, consider $(t_1(h), t_2(h)) \in \wc_0 = Adv_1 \times Coop_2$. By construction of $\T$, it follows that $h$ is a legal history such that $h \models \varphi_1$ and $h \models \varphi_2$. In $(t_1(h), t_2(h))$, we have that $\sigma$ is undefined, i.e., it stops, and achieves $\val{(\varphi_1, \varphi_2)|\P}(\sigma, h) = \langle \win, \win \rangle$. 

Then, if $(t_1(h), t_2(h)) \in \wc_{i}$, then $\val{(\varphi_1, \varphi_2)|\P}(\sigma, h) \in \{\langle \win, \win \rangle, \langle \win, \pend \rangle\}$ is the inductive hypothesis. Assume that $(t_1(h), t_2(h)) \in \wc_{i+1} \setminus \wc_{i}$ (as otherwise the claim would be trivially true by the inductive hypothesis). To prove that $\val{(\varphi_1, \varphi_2)|\P}(\sigma, h) \in \{\langle \win, \win \rangle, \langle \win, \pend \rangle\}$ we prove separately that: \myi~$\val{\varphi_1|\P}(\sigma, h) = \win$, and \myii~$\val{\varphi_2|\P}(\sigma, h) \in \{\win, \pend\}$.

We prove \myi. By the fixpoint computation in Lines~7 and~8 of Algorithm~\ref{alg:strong-weak-plan}, we have that in $(t_1(h), t_2(h))$, where the agent strategy plays an action $\hat{a}$ defined as in Step~9 (case 1), there are two possibilities depending on the environment reaction $r$: \begin{compactenum}
        \item[(a)] The successor state $(t'_1(h'), t'_2(h')) = (\partial((t_1(h), t_2(h))), \hat{a}, r) \in \wc_i$, in which case $h' \in \H_{\P}(\sigma)$, and, by the inductive hypothesis, $\val{\langle \varphi_1, \varphi_2 \rangle|\P}(\sigma, h') = \langle \win, \pend \rangle$, and hence $\val{\varphi_1|\P}(h') = \win$; or
        \item[(b)] $(t'_1(h'), t'_2(h')) = (\partial((t_1(h), t_2(h))), \hat{a}, r) \in \w_1 \times \overline{\c_2}$, in which case $h' \in \H_{\P}(\sigma)$ and, by construction of $\T$, we have that  $(t'_1(h'), t'_2(h')) \in \w_1$. By Item 1 Lemma~\ref{lem:games-to-histories}, $\val{\varphi_1|\P}(\kappa_1, h') = \win$. From $(t'_1(h'), t'_2(h'))$, $\sigma$ always follows $\kappa_1$, hence achieving $\val{\varphi_1|\P}(\sigma, h') = \win$. 
    \end{compactenum}
    By Items~(a) and~(b) above, 
    we have that $\sigma$ achieves $\val{\varphi_1|\P}(\sigma, h') = \win$ in every extension $h'$ of $h$. As a result, $\sigma$ achieves $\val{\varphi_1|\P}(\sigma, h) = \win$.

    We prove \myii. By the fixpoint computation in Lines~7 and~8 of Algorithm~\ref{alg:strong-weak-plan}, there exists an agent action, say $\hat{a}$, and an environment reaction, say $\hat{r}$, such that $(t'_1(h'), t'_2(h')) = (\partial((t_1(h), t_2(h))), \hat{a}, \hat{r}) \in \wc_i$. By Line~9 in Algorithm~\ref{alg:strong-weak-plan}, $\sigma$ prescribes one such action $\hat{a}$. By construction of $\T$, we have that $(t'_1(h'), t'_2(h'))$ corresponds to an history $h' \in \H_{\P}(\sigma)$ that extends $h$. By the inductive hypothesis, $\val{(\varphi_1, \varphi_2)|\P}(\sigma, h') \in \{\langle \win, \win \rangle, \langle \win, \pend \rangle\}$, meaning that $\val{\varphi_2|\P}(h') \in \{\win, \pend\}$. 
    Since the agent can extend $h$ into $h'$ satisfying $\val{\varphi_2|\P}(h') \in \{\win, \pend\}$ (with the agent action $\hat{a}$ and the environment reaction $\hat{r}$), we have $\sigma$ achieves at least $\val{\varphi_2|\P}(\sigma, h) = \pend$, so that \myii holds.  
    
    $(\dagger)$ follows from \myi and \myii.

    We now prove Item 2. Let $(t_1(h), t_2(h)) \in \wc \cap (\w_1 \times (\c_2 \setminus \w_2))$. We have that $\val{\langle\varphi_1,\varphi_2\rangle|\P}(\sigma, h) \in \{\langle \win, \win \rangle, \langle \win, \pend \rangle\}$ by $(\dagger)$. By Item 1 Lemma~\ref{lem:strong-weak-plans}, if  $\val{\langle \varphi_1, \varphi_2 \rangle|\P}(h) = \langle\win, \pend\rangle$, then $(t_1(h), t_2(h)) \in \w_1 \times (\c_2 \setminus \w_2)$. Then, it follows by definition of value that $\val{\langle\varphi_1,\varphi_2\rangle|\P}(\sigma, h) = \langle \win, \pend \rangle$.

    We prove Item 3. We begin with \textbf{(A)}. To do so, we prove the contradiction. That is, suppose that there exists an agent strategy $\eta$ such that $\val{(\varphi_1, \varphi_2)|\P}(\eta, h) = \langle \win, \pend \rangle$. We will prove that $(t_1(h), t_2(h)) \not \in (\w_1 \times (\c_2 \setminus \w_2)) \setminus \wc$. Since $\val{(\varphi_1, \varphi_2)|\P}(\eta, h) = \langle \win, \pend \rangle$, the following must hold: $\val{(\varphi_1, \varphi_2)|\P}(h) = \{\langle \win, \win \rangle, \langle \win, \pend \rangle\}$, i.e., either there exists a strategy that wins both $\varphi_1$ and $\varphi_2$, or one that wins $\varphi_1$ and possibly wins $\varphi_2$ (with $\eta$ being a strategy that witnesses this latter case). 
    
    First, suppose that $\val{(\varphi_1, \varphi_2)|\P}(h) = \langle \win, \win \rangle$. By Item~1 in Lemma~\ref{lem:games-to-histories}, we have $t_1(h) \in \w_1$ and $t_2(h) \in \w_2$. As a result $(t_1(h), t_2(h)) \in \w_1 \times \w_2$, meaning that $(t_1(h), t_2(h)) \not \in \w_1 \times (\c_2 \setminus \w_2)$. Hence, $(t_1(h), t_2(h)) \not \in (\w_1 \times (\c_2 \setminus \w_2)) \setminus \wc$. 
    
    Suppose now that $\val{(\varphi_1, \varphi_2)|\P}(h) = \langle \win, \pend \rangle$. Since $\val{(\varphi_1, \varphi_2)|\P}(\eta, h) = \langle \win, \pend \rangle$, it follows by definition of value that, for every legal environment strategy $\gamma \in \Gamma_{\P}(\sigma, h)$, we have $\Play(\eta, \gamma) \models_{\P} \varphi_1$, and there exists a legal environment strategy, say $\hat{\gamma} \in \Gamma_{\P}(\sigma, h)$, such that $\Play(\eta, \hat{\gamma}) \models_{\P} \varphi_2$. By construction of $\T_1$, it follows that, for every environment strategy, $\Play(\eta, \gamma)$ is accepted by $(\T^{t_1(h)}_1, Adv_1)$, where $\T^{t_1(h)}_1$ is as $\T_1$, but with the new initial state $t_1(h)$, hence $t_1(h)$ is a winning state in $\w_1$. By construction of $\T_2$, we have instead that $\Play(\eta, \hat{\gamma})$ is accepted by$ (\T^{t_2(h)}_1, Coop_2)$, where $\T^{t_2(h)}_2$ is as $\T_2$, but with the new initial state  $t_2(h)$. Hence $t_2(h)$ is a winning state in $\c_2$. However, $t_2(h) \not \in \w_2$, since $\val{\varphi_2|\P}(\eta, h) = \pend$). As a result $(t_1(h), t_2(h)) \in \w_1 \times (\c_2 \setminus \w_2)$. To prove the contradiction we need to show that $(t_1(h), t_2(h)) \in \wc$. To see this, observe that, since $\T$ is obtained by product of $\T_1$ and $\T_2$, $\Play(\eta, \hat{\gamma})$ is accepted by $(\T^{(t_1(h), t_2(h))}, Adv_1 \times Coop_2)$, where $\T^{(t_1(h), t_2(h))}$ is as $\T$, but with the new initial state ${(t_1(h), t_2(h))}$. Furthermore, Since $\eta$ never leaves the winning region $\w_1$ (otherwise $\val{\varphi_1|\P}(\eta, h) \neq \win$), it follows by the definition of the fixpoint computation in Lines~7 and~8 of Algorithm~\ref{alg:strong-weak-plan}, that $(t_1(h), t_2(h)) \in \wc$, which proves the contradiction.

    We now prove \textbf{(B)}. Since $(t_1(h), t_2(h)) \in (\w_1 \times (\c_2 \setminus \w_2)) \setminus \wc$, it follows by construction of $\T'$ that $t_1(h) \in \w_1$. By Item~3 Lemma~\ref{lem:games-to-histories}, $\val{\varphi_1|\P}(\kappa_1, h) = \win$. By Step~9 in Algorithm~\ref{alg:strong-weak-plan}, $\sigma$ always follows $\kappa_1$ from $(t_1(h), t_2(h))$ onwards. As a result $\val{\varphi_1|\P}(\sigma, h) = \win$.    
\end{proof}

With Lemma~\ref{lem:strong-weak-plans} in place, we are ready to prove Theorem~\ref{thm:win-pend-strategy}. 

\begin{proof}[Proof of Theorem~\ref{thm:win-pend-strategy}] Let $h \in \H_{\P}(\sigma)$ be an history such that $\val{(\varphi_1, \varphi_2)|\P}(h) = \langle \win, \pend \rangle$. By Item 1 Lemma~\ref{lem:strong-weak-plans}, $(t_1(h), t_2(h)) \in \w_1 \times (\c_2 \setminus \w_2)$. Now, observe that $\wc \cap (\w_1 \times (\c_2 \setminus \w_2))$ and $(\w_1 \times (\c_2 \setminus \w_2)) \setminus \wc$  partition $(\w_1 \times (\c_2 \setminus \w_2))$. Then, one of the two holds: (a) $(t_1(h), t_2(h)) \in \wc \cap (\w_1 \times (\c_2 \setminus \w_2))$, or (b) $(t_1(h), t_2(h)) \in (\w_1 \times (\c_2 \setminus \w_2)) \setminus \wc$. Suppose (a) holds. Then, by Item 2 Lemma~\ref{lem:strong-weak-plans}, $\val{(\varphi_1,\varphi_2)|\P}(\sigma, h) = \langle \win, \pend \rangle$, so that Item 1 in Theorem~\ref{thm:win-pend-strategy} holds. Else, suppose (b) holds. Then, by Item 3 Lemma~\ref{lem:strong-weak-plans}, no agent strategy $\eta$ exists such that $\val{(\varphi_1, \varphi_2)}(\eta, h) = \langle \win, \pend \rangle$ and $\val{\varphi_1}(\sigma, h) = \win$, so that Item 2 in Theorem~\ref{thm:win-pend-strategy} holds.
\end{proof}

\subsection{Proof of Theorem~\ref{thm:multi-tier-correct}}

% cosa facciamo di preciso in questa sezione?
In what follows, we present the proof of Theorem~\ref{thm:multi-tier-correct}, i.e., correctness of Algorithm~\ref{alg:super-mega-iper-ultra-multi-tier}. 
% che cosa dobbiamo fare di preciso?
That amounts to show that the strategy returned by Algorithm~\ref{alg:super-mega-iper-ultra-multi-tier} always satisfies Definition~4, which we report below for convenience.

\setcounter{definition}{+3}
\begin{definition}[Adaptive Strategy for Multi-Tier Goals]~\label{def:best-effort-plan}
    Let $\P$ be a nondeterministic planning domain and $\Phi = \langle \varphi_1, \cdots, \varphi_n \rangle$ a multi-tier goal. An agent strategy $\sigma$ is an adaptive strategy for $\Phi$ in $\P$ if, for every $h \in \H_{\P}(\sigma)$, one of the following holds: 
    \begin{enumerate}[noitemsep,topsep=0pt,parsep=0pt,partopsep=0pt]
        \item 
        Suppose both the maximally winning objective $\varphi_{\ell}$ and the maximally winning-pending objective $\varphi_k$
        % in $\P$ 
        exist, then: \myi $\sigma$ is winning for $\varphi_\ell$ in $\P$ from $h$, and \myii there exists an agent strategy $\sigma'$ such that $\val{\varphi_k|\P}(\sigma', h) = \pend$ and $\sigma(h) = \sigma'(h)$ % \myii there exists an agent strategy $\sigma'$ such that $\val{\langle \varphi_{\ell}, \varphi_k \rangle|\P}(\sigma', h) = \langle \win, \pend \rangle$ and $\sigma(h) = \sigma'(h)$;
        % \gp{Should it not be \myii there exists an agent strategy $\sigma'$ such that $\val{\varphi_k|\P}(\sigma', h) = \pend$ and $\sigma(h) = \sigma'(h)$?}
        \item 
        Suppose the maximally winning objective  $\varphi_{\ell}$ 
        exists, yet no maximally winning-pending 
        exists, then $\sigma$ is winning for $\varphi_{\ell}$ in $\P$ from $h$;
        \item 
        Suppose neither the maximally winning objective nor the maximally winning-pending objective exists, yet there exists a maximally pending objective $\varphi_{p}$, then there exists an agent strategy $\sigma'$ such that $val_{\varphi_p|\P}(\sigma', h) = \pend$ and $\sigma(h) =  \sigma'(h)$. % $\sigma$ is pending for $\varphi_{p}$ in $\P$.
        % \item 
        % Suppose none of the above holds, $\sigma(h)$ just returns any legal action. 
    \end{enumerate}
\end{definition}

\begin{theorem}~\label{thm:multi-tier-correct}
    % Let $\P$ be a domain and $\Phi$ a multi-tier goal. 
    Alg.~\ref{alg:super-mega-iper-ultra-multi-tier} %orithm~\ref{alg:super-mega-iper-ultra-multi-tier} 
    returns an adaptive strategy for $\Phi$ in $\P$.
    % Strategy $\sigma$ returned by Algorithm~\ref{alg:super-mega-iper-ultra-multi-tier} is an adaptive strategy for $\Phi$ in $\P$.
\end{theorem}

\begin{proof}[Proof of Theorem~\ref{thm:multi-tier-correct}]
Consider $h \in \H_{\P}(\sigma)$. We prove that $\sigma$ behaves as prescribed in every item of Definition~\ref{def:best-effort-plan}. 

We consider first the case where the maximally winning objective wrt $h$ is $\varphi_j$ and no maximally winning-objective wrt exists.
By Item 2, Definition~\ref{def:best-effort-plan}, we need to prove that $\sigma$ is winning for $\varphi_j$ from $h$. Being $\varphi_j$ the maximally winning objectives with respect to $h$, we have that $q'_j \in \w_j$ and $j = max\{i \tst q'_i \in \w_i\}$. We have that $\sigma$ follows $\kappa_j$ in $h$ and all its extensions $h' \in \H_{\P}(\sigma)$, as no other objective $\varphi_\ell$ (with $\ell > j$) can be achieved from $h$. Being $\kappa_j$ winning for $\varphi_j$ from $h$, we have that $\sigma$ is winning for $\varphi_j$ from $h$ as well. The case where no maximally winning objective and maximally winning-pending exist, yet there exists a maximally pending objective, is similar. 

% quale è di preciso il caso che consideriamo?
Suppose the maximally winning and maximally winning-pending objectives wrt $h$ are $\varphi_j$ and $\varphi_\ell$ ($\ell > j$), respectively. By Item 1, Definition~\ref{def:best-effort-plan}, we need to prove that $\sigma$ is winning for $\varphi_j$ and follows a strategy that cooperates for $\varphi_\ell$ in $h$.
We prove the claim by backward induction from $n-1$ to $1$ 
% cosa accade di preciso al caso n
(in fact, if $\varphi_n$ is the maximally winning objective, no maximally winning-pending objective exists). 
%     For Item 1, we proceed by backward induction from $n-1$ to $1$, where $n$ is the number of objectives in $\Phi$ (the case $n$ is handled in Item 1). 
For the base case, suppose $\varphi_{n-1}$ is the maximally winning objective wrt $h$, and $\varphi_{n}$ is the maximally winning-pending goal wrt $\varphi_{n-1}$ and $h$. By definition, there exists a strategy $\omega$ s.t. $\val{(\varphi_{n-1}, \varphi_{n})|\P}(\omega, h) = \langle \win, \pend \rangle$.
Then, $n-1 = \{i \tst q'_i \in \w_i\}$ and $n = \max\{i \tst i > n-1 \text{ and } q'_i \in \wc_{(n-1,i)}\}$. As a result, $\sigma$ follows $\omega$ in $h$, so that \myii in Item 1 holds. For \myi, observe that, $\sigma$ will eventually switch to another agent strategy and, in every extension $h' \in \H_{\P}(\sigma)$ of $h$ where $\sigma$ does not follow $\omega$, we have either: \textbf{(A)} $\val{(\varphi_{n-1}, \varphi_{n})|\P}(h') = \langle \win, \win \rangle$, i.e., the environment cooperated and $\varphi_n$ is the maximal winning objective wrt $h'$, or \textbf{(B)} $\val{(\varphi_{n-1}, \varphi_n)|\P}(h') = \langle \win, \lose \rangle$, i.e., the environment did not cooperative and $\varphi_{n-1}$ is the maximal winning objective wrt $h'$ and no maximal winning-pending objective wrt $\varphi_{n-1}$ and $h'$ exists. If \textbf{(A)} holds, $\sigma$ follows $\kappa_n$ and satisfies $\varphi_n$, which implies $\varphi_{n-1}$ by our assumption that $\Phi$ is a multi-tier goal. If \textbf{(B)} holds, $\sigma$ follows $\kappa_{n-1}$ and satisfies $\varphi_{n-1}$. As a result, $\sigma$ is winning for $\varphi_{n-1}$ from $h$ and \myi in Item 1 holds. 

The inductive step is similar. Assume $\varphi_i$ is the maximally winning object wrt $h$ and $\varphi_{j}$ (for $j > i$) is the maximally winning-pending goal wrt $\varphi_i$ and $h$. The argument for \myii in Item 1 is the same as above and $\sigma$ follows $\omega_{ij}$ such that $\val{(\varphi_i, \varphi_j)|\P}(\omega_{ij}, h) = \langle \win, \pend \rangle$ in $h$. 
As for \myi, observe that in some $h' \in \H_{\P}(\sigma)$, $\sigma$ will switch to another agent strategy. By the inductive hypothesis, we have that, regardless of how it switches, $\sigma$ wins $\varphi_i$ from $h$.
\end{proof}
